# Supplementary material for: RobustNav: Towards Benchmarking Robustness in Embodied Navigation
Source: arXiv:2106.04531 source file (2021-06-08)
Supplement: Supplementary file 1 [file traj_vis.tex]

We also provide visualizations of trajectories executed by \pnav and \onav agents
under clean and corrupt settings. These are present as videos -- named \verb|pnav_rgb.mp4| (for \pnav \texttt{RGB}), \verb|pnav_rgbd.mp4| (for \pnav \texttt{RGBD}), \verb|onav_rgb.mp4| (for \onav \texttt{RGB}) and
\verb|onav_rgbd.mp4| (for \onav \texttt{RGBD}).
For each episode, we show the ego-centric RGB (on the left), depth
(in the middle if applicable)
and top-down (on the right) views. The goal object / location is highlighted via a blue circle in the top-down
views.

\clearpage
